# Supplementary material for: Autonomous Embodied Agents: When Robotics Meets Deep Learning Reasoning
Source: arXiv:2505.00935 source file (2025-05-02)
Supplement: Supplementary file 1 [file tab3.tex]

\begin{table*}[t!]
\centering
\label{tab:mp3d_val_results}
\setlength{\tabcolsep}{.35em}
\resizebox{0.95\linewidth}{!}{
\begin{tabular}{lc ccccccccc}
\toprule
 & & \multicolumn{9}{c}{\textbf{Estimated Localization}} \\
\cmidrule{3-11}
 & & $\mathsf{Seen [\%]}$ & $\mathsf{Acc.}$ & $\mathsf{IoU}_{+}$ & $\mathsf{IoU}_{-}$ & $\mathsf{IoU}$ & $\mathsf{mAcc.}$ & $\mathsf{mIoU}_{+}$ & $\mathsf{mIoU}_{-}$ & $\mathsf{mIoU}$ \\
\midrule
\textbf{OccAnt}$^\dagger$   & & 50.3 & 24.1 & 9.6 & 5.8 & 8.5 & 49.5 & 13.9 & 7.0 & 11.6\\
\midrule
\textbf{DR} & & 48.0 & 28.7 & 11.9 & 7.3 & 10.7 & 59.7 & 17.3 & 9.0 & 14.7\\
\textbf{AR} & & 40.1 & 29.4 & 15.9 & 13.0 & 15.7 & 71.3 & 28.8 & \textbf{16.8} & 25.9\\
\textbf{CR} & & \textbf{53.2} & 34.7 & 14.6 & 8.7 & 12.9 & 64.1 & 20.3 & 10.3 & 17.0\\
\midrule
\textbf{AR+DR}  & & 48.7 & 34.9 & 16.6 & 11.9 & 15.7 & 71.7 & 26.7 & 14.2 & 22.9\\
\textbf{CR+DR}  & & 50.1 & \textbf{38.6} & \textbf{20.1} & \textbf{14.1} & \textbf{19.1} & \textbf{75.4} & \textbf{31.8} & \textbf{16.8} & \textbf{27.6}\\

\midrule
                
 & & \multicolumn{9}{c}{\textbf{Oracle Localization}}\\
\cmidrule{3-11}
 & & $\mathsf{Seen [\%]}$ & $\mathsf{Acc.}$ & $\mathsf{IoU}_{+}$ & $\mathsf{IoU}_{-}$ & $\mathsf{IoU}$ & $\mathsf{mAcc.}$ & $\mathsf{mIoU}_{+}$ & $\mathsf{mIoU}_{-}$ & $\mathsf{mIoU}$\\
\midrule
\textbf{OccAnt}$^\dagger$   & & 47.5 & 33.5 & 21.5 & 17.4 & 20.6 & 76.0 & 41.6 & 23.0 & 20.1 \\
\midrule
\textbf{DR} & & 44.7 & 35.2 & 22.3 & 19.0 & 22.1 & 79.4 & 42.4 & 25.0 & 38.2 \\
\textbf{AR} & & 39.2 & 31.0 & 19.2 & 17.7 & 19.4 & 77.6 & 38.9 & 24.8 & 36.0 \\
\textbf{CR} & & \textbf{52.2} & \textbf{42.6} & \textbf{26.9} & 19.8 & \textbf{25.4} & 80.4 & \textbf{46.4} & 25.2 & \textbf{40.2} \\
\midrule
\textbf{AR+DR}  & & 47.6 & 38.0 & 22.6 & 19.3 & 22.4 & \textbf{81.3} & 42.0 & 25.4 & 37.5 \\
\textbf{CR+DR}  & & 50.0 & 40.9 & 25.1 & \textbf{19.9} & 24.3 & 80.8 & 43.8 & \textbf{26.2} & 39.2 \\
\bottomrule
\end{tabular}
}
\caption{Experimental results on MP3D validation set.} 
\label{tab:tab3_sd}
% \label{tab:mp3d_val_results}
\end{table*}
