# Supplementary material for: Autonomous Embodied Agents: When Robotics Meets Deep Learning Reasoning
Source: arXiv:2505.00935 source file (2025-05-02)
Supplement: Supplementary file 2 [file tab4.tex]

\begin{table}[t!]
\centering
\setlength{\tabcolsep}{.35em}
\resizebox{.95\linewidth}{!}{
\begin{tabular}{lc ccccccccc}
\toprule
 & & \multicolumn{9}{c}{\textbf{Oracle Localization}}\\
\cmidrule{3-11}
 & & $\mathsf{Seen [\%]}$ & $\mathsf{Acc.}$ & $\mathsf{IoU}_{+}$ & $\mathsf{IoU}_{-}$ & $\mathsf{IoU}$ & $\mathsf{mAcc.}$ & $\mathsf{mIoU}_{+}$ & $\mathsf{mIoU}_{-}$ & $\mathsf{mIoU}$  \\
\midrule
\textbf{OccAnt} & & 81.6 & 60.1 & \textbf{32.1} & 21.2 & 29.2 & 78.7 & \textbf{39.6} & 22.2 &  \textbf{34.1} \\
\midrule
\textbf{DR} & & \textbf{86.1} & \textbf{65.2} & 30.1 & \textbf{24.1} & \textbf{29.9} & 81.1 & 36.0 & 25.2 & 33.8 \\
\textbf{AR} & & 74.1 & 53.8 & 27.9 & 21.9 & 27.2 & 77.0 & 35.4 & 23.5 & 32.7 \\
\textbf{CR} & & 84.0 & 62.2 & 30.6 & 22.1 & 28.8 & 79.5 & 36.1 & 23.3 & 32.8 \\
\midrule
\textbf{AR+DR}  & & 83.2 & 63.2 & 29.6 & 23.8 & 29.1 & \textbf{81.6} & 35.8 & 25.1 & 33.7 \\
\textbf{CR+DR}  & & 82.6 & 63.8 & 30.3 & \textbf{24.1} & 29.5 & \textbf{81.6} & 36.1 & \textbf{25.5} & 34.0 \\
\bottomrule
\end{tabular}
}
\caption{Experimental results on Gibson validation set using the oracle localization setup.}
\label{tab:tab4_sd}
% \label{tab:gibson_oracle_results}
\end{table}
